# Supplementary material for: The COLIBRE project: cosmological hydrodynamical simulations of galaxy formation and evolution
Source: arXiv:2508.21126 ancillary file (2026-02-22)
Supplement: Supplementary file 1 [file output_properties.pdf]

| Particle type | Field Name                      | Description                                                                                                                                                              | Snipshots |
|---------------|---------------------------------|--------------------------------------------------------------------------------------------------------------------------------------------------------------------------|-----------|
| DM            | Coordinates                     | Co-moving position of the particles                                                                                                                                      | ✓         |
| DM            | FOFGroupIDs                     | Friends-Of-Friends ID of the group the particles belong to                                                                                                               | ✓         |
| DM            | Masses                          | Masses of the particles                                                                                                                                                  | ✓         |
| DM            | ParticleIDs                     | Unique ID of the particles                                                                                                                                               | ✓         |
| DM            | Potentials                      | Gravitational potentials of the particles                                                                                                                                | ✓         |
| DM            | Velocities                      | Peculiar velocities of the particles. This is a * dx/dt where x is the co-moving position of the particles.                                                              | ✓         |
| Gas           | AveragedStarFormationRates      | Star formation rates of the particles averaged over the period set by the first two snapshot triggers                                                                    | ✗         |
| Gas           | ComptonYParameters              | Compton y parameters in the physical frame computed based on the cooling tables. This is 0 for star-forming particles.                                                   | ✗         |
| Gas           | Coordinates                     | Co-moving positions of the particles                                                                                                                                     | ✓         |
| Gas           | Densities                       | Co-moving mass densities of the particles                                                                                                                                | ✓         |
| Gas           | DensitiesAtLastAGNEvent         | Physical density (not subgrid) of the gas at the last AGN feedback event that hit the particles. -1 if the particles have never been heated.                             | ✗         |
| Gas           | DensitiesAtLastSupernovaEvent   | Physical density (not subgrid) of the gas at the last SN (type-II or type-Ia) thermal feedback event that hit the particles. -1 if the particles have never been heated. | ✗         |
| Gas           | DiffusionParameters             | Diffusion coefficient (alpha_diff) of the particles                                                                                                                      | ✗         |
| Gas           | DustMassFractions               | Fractions of the particles' masses that are in a given species of dust grain                                                                                             | ✗         |
| Gas           | ElementMassFractions            | Fractions of the particles' masses that are in the given element                                                                                                         | ✗         |
| Gas           | ElementMassFractionsDiffuse     | Fractions of the particles' masses that are in the given element and in the diffuse (non-dust) phase                                                                     | ✗         |
| Gas           | EnergiesReceivedFromAGNFeedback | Total amount of thermal energy from AGN feedback events received by the particles.                                                                                       | ✗         |
| Gas           | Entropies                       | Co-moving entropies per unit mass of the particles                                                                                                                       | ✗         |
| Gas           | FOFGroupIDs                     | Friends-Of-Friends ID of the group the particles belong to                                                                                                               | ✓         |

|     |                                      |                                                                                                                                                                                                                                                     |   |
|-----|--------------------------------------|-----------------------------------------------------------------------------------------------------------------------------------------------------------------------------------------------------------------------------------------------------|---|
| Gas | InternalEnergies                     | Co-moving thermal energies per unit mass of the particles                                                                                                                                                                                           | ✓ |
| Gas | IronMassFractionsFromSNIa            | Fractions of the particles' masses that are in iron produced by SNIa stars (incorporating both depleted and nebular phases)                                                                                                                         | × |
| Gas | IronMassFractionsFromSNIaDiffuse     | Fractions of the particles' masses that are in iron originating from SNIa, but not depleted into dust                                                                                                                                               | × |
| Gas | LaplacianInternalEnergies            | Laplacian (del squared) of the Internal Energy per unit mass of the particles                                                                                                                                                                       | × |
| Gas | LastAGNFeedbackScaleFactors          | Scale-factors at which the particles were last hit by AGN feedback. -1 if a particle has never been hit by feedback                                                                                                                                 | ✓ |
| Gas | LastEnergiesReceivedFromAGNFeedback  | The energy the particles received the last time they were heated by AGN feedback.                                                                                                                                                                   | × |
| Gas | LastFOFHaloMasses                    | Masses of the last FOF haloes the particles where part of. -1 if the particle has never been in a FOF group                                                                                                                                         | × |
| Gas | LastFOFHaloMassesScaleFactors        | Scale-factors at which the particle was last in a FOF group                                                                                                                                                                                         | × |
| Gas | LastISMScaleFactors                  | Scale-factor at which the particle was part of the ISM for the last time, i.e. its density was larger than 100 times the mean density and (its neutral fraction larger than 50% OR be an HII region). -1 if the particle was never part of the ISM. | ✓ |
| Gas | LastKineticEarlyFeedbackScaleFactors | Scale-factors at which the particles were last hit by kinetic early feedback. -1 if a particle has never been hit by feedback                                                                                                                       | × |
| Gas | LastSNIKineticFeedbackScaleFactors   | Scale-factors at which the particles were last hit by SNII kinetic feedback. -1 if a particle has never been hit by feedback                                                                                                                        | × |
| Gas | LastSNIKineticFeedbackvkick          | Physical kick velocity the particles were kicked with at last SNII kinetic feedback event. -1 if a particle has never been hit by feedback                                                                                                          | × |

|     |                                     |                                                                                                                                        |   |
|-----|-------------------------------------|----------------------------------------------------------------------------------------------------------------------------------------|---|
| Gas | LastSNIIThermalFeedbackScaleFactors | Scale-factors at which the particles were last hit by SNI thermal feedback. -1 if a particle has never been hit by feedback            | ✓ |
| Gas | LastSNIaThermalFeedbackScaleFactors | Scale-factors at which the particles were last hit by SNIa thermal feedback. -1 if a particle has never been hit by feedback           | × |
| Gas | LastStarFormationScaleFactors       | Scale-factors at which the stars last had a non-zero star formation rate.                                                              | × |
| Gas | MassFractionsFromAGB                | Fractions of the particles' masses that have been produced by AGN stars                                                                | × |
| Gas | MassFractionsFromCEJSN              | Fractions of the particles' masses that have been produced by common-envelop jets SN events                                            | × |
| Gas | MassFractionsFromCollapsar          | Fractions of the particles' masses that have been produced by collapsar events                                                         | × |
| Gas | MassFractionsFromNSM                | Fractions of the particles' masses that have been produced by neutron star merger events                                               | × |
| Gas | MassFractionsFromSNII               | Fractions of the particles' masses that have been produced by SNII stars                                                               | × |
| Gas | MassFractionsFromSNIa               | Fractions of the particles' masses that have been produced by SNIa stars                                                               | × |
| Gas | Masses                              | Masses of the particles                                                                                                                | ✓ |
| Gas | MaximalSNIKineticFeedbackvkick      | Maximal physical kick velocity the particles were kicked with in SNI kinetic feedback. -1 if a particle has never been hit by feedback | × |
| Gas | MaximalTemperatureScaleFactors      | Scale-factors at which the maximal temperature was reached                                                                             | × |
| Gas | MaximalTemperatures                 | Maximal temperatures ever reached by the particles                                                                                     | × |
| Gas | MeanIronWeightedRedshifts           | Mean redshift of SNIa events weighted by the iron mass imparted by each event. -1 if a particle has never been enriched by SNIa.       | × |
| Gas | MeanMetalWeightedRedshifts          | Mean redshift of enrichment events weighted by the metal mass imparted by each event. -1 if a particle has never been enriched.        | × |
| Gas | MetalMassFractions                  | Fractions of the particles' masses that are in metals (incorporating both depleted and nebular phases)                                 | ✓ |

|     |                                    |                                                                                                                                                                                                                                                                                            |   |
|-----|------------------------------------|--------------------------------------------------------------------------------------------------------------------------------------------------------------------------------------------------------------------------------------------------------------------------------------------|---|
| Gas | MetalMassFractionsFromAGB          | Fractions of the particles' masses that are in metals produced by AGB stars (incorporating both depleted and nebular phases)                                                                                                                                                               | × |
| Gas | MetalMassFractionsFromSNII         | Fractions of the particles' masses that are in metals produced by SNII stars (incorporating both depleted and nebular phases)                                                                                                                                                              | × |
| Gas | MetalMassFractionsFromSNIa         | Fractions of the particles' masses that are in metals produced by SNIa stars (incorporating both depleted and nebular phases)                                                                                                                                                              | × |
| Gas | MinimalSmoothingLengthScaleFactors | Scale-factors at which the minimal smoothing length was reached                                                                                                                                                                                                                            | × |
| Gas | MinimalSmoothingLengths            | Minimal smoothing lengths ever reached by the particles                                                                                                                                                                                                                                    | × |
| Gas | ParticleIDs                        | Unique IDs of the particles                                                                                                                                                                                                                                                                | ✓ |
| Gas | Potentials                         | Co-moving gravitational potential at position of the particles                                                                                                                                                                                                                             | × |
| Gas | Pressures                          | Co-moving pressures of the particles                                                                                                                                                                                                                                                       | ✓ |
| Gas | ProgenitorParticleIDs              | ID of the progenitor of this particle. If this particle is the result of one (or many) splitting events, this ID corresponds to the ID of the particle in the initial conditions that its lineage can be traced back to. If the particle was never split, this is the same as ParticleIDs. | ✓ |
| Gas | SmoothingLengths                   | Co-moving smoothing lengths (FWHM of the kernel) of the particles                                                                                                                                                                                                                          | ✓ |
| Gas | SpeciesFractions                   | Species fractions array for all ions and molecules in the CHIMES network. The fraction of species $i$ is defined in terms of its number density relative to hydrogen, i.e. $n_i / n_{H_{tot}}$ .                                                                                           | × |
| Gas | SplitCounts                        | Number of times this particle has been split. Note that both particles that take part in the splitting have their counter incremented.                                                                                                                                                     | ✓ |
| Gas | SplitTrees                         | Binary tree describing splitting events. Particles that keep the original ID have a value of zero in a splitting event, whereas particles given a new ID have a value of one.                                                                                                              | ✓ |

|     |                                          |                                                                                                                                                                                                                                                                                                                                                     |   |
|-----|------------------------------------------|-----------------------------------------------------------------------------------------------------------------------------------------------------------------------------------------------------------------------------------------------------------------------------------------------------------------------------------------------------|---|
| Gas | StarFormationRates                       | Star formation rates of the particles.                                                                                                                                                                                                                                                                                                              | ✓ |
| Gas | TemperatureIncreasesAtLastAGNEvent       | The increase in temperature of the gas at the last AGN feedback event that hit the particles. -1 if the particles have never been heated.                                                                                                                                                                                                           | ✓ |
| Gas | TemperatureIncreasesAtLastSupernovaEvent | The increase in temperature of the gas at the last SN (type-II or type-Ia) thermal feedback event that hit the particles. -1 if the particles have never been heated.                                                                                                                                                                               | ✓ |
| Gas | Temperatures                             | Temperature of the particles                                                                                                                                                                                                                                                                                                                        | ✓ |
| Gas | TotalDustMassFractions                   | Fractions of the particles' masses that are in dust (sum of all grains species)                                                                                                                                                                                                                                                                     | ✓ |
| Gas | TotalElectronNumberDensities             | Total electron number densities in the physical frame computed as the sum of the electron number densities from the elements evolved with the non-equilibrium network CHIMES and the electron number densities from the other elements based on the equilibrium cooling tables.                                                                     | ✓ |
| Gas | Velocities                               | Peculiar velocities of the stars. This is $(a * dx/dt)$ where x is the co-moving positions of the particles                                                                                                                                                                                                                                         | ✓ |
| Gas | VelocityDispersions                      | Physical velocity dispersions (3D) squared, this is the velocity dispersion of the total velocity (peculiar velocity + Hubble flow, $a H x + a (dx/dt)$ ). Values of the Velocity dispersion that have the value of FLT_MAX are particles that do not have neighbours and therefore the velocity dispersion of these particles cannot be calculated | × |
| Gas | VelocityDivergenceTimeDifferentials      | Time differential (over the previous step) of the velocity divergence field around the particles. Again, provided without cosmology as this includes a Hubble flow term.                                                                                                                                                                            | × |
| Gas | VelocityDivergences                      | Local velocity divergence field around the particles. Provided without cosmology, as this includes the Hubble flow.                                                                                                                                                                                                                                 | × |
| Gas | ViscosityParameters                      | Viscosity coefficient ( $\alpha_{\text{visc}}$ ) of the particles, multiplied by the balsara switch                                                                                                                                                                                                                                                 | × |

|              |                                         |                                                                                                                                                                                                                                                                        |   |
|--------------|-----------------------------------------|------------------------------------------------------------------------------------------------------------------------------------------------------------------------------------------------------------------------------------------------------------------------|---|
| Gas          | XrayLuminosities                        | Intrinsic X-ray luminosities in various bands. This is 0 for star-forming particles.                                                                                                                                                                                   | × |
| Gas          | XrayPhotonLuminosities                  | Intrinsic X-ray photon luminosities in various bands. This is 0 for star-forming particles.                                                                                                                                                                            | × |
| Gas (Hybrid) | EnergiesReceivedFromJetFeedback         | Total amount of kinetic energy from AGN jet feedback events received by the particles.                                                                                                                                                                                 | × |
| Gas (Hybrid) | InternalEnergyViscousTimeDifferentials  | Co-moving time differentials of the internal energy (per unit mass) due to artificial viscosity. This is the rate at which particles are converting their specific kinetic energy to internal energy due to shocks.                                                    | × |
| Gas (Hybrid) | JetRadioEmissionGammaEffectiveIntegrals | Integrals over the gamma integrals, which are used to compute values weighted by the shock injection rates as a function of time. These are in physical frame.                                                                                                         | × |
| Gas (Hybrid) | JetRadioEmissionGammaIntegrals          | Integrals over the synchrotron photon and CMB photon energy densities, respectively, in physical frame. These are used for radio emission modeling (see documentation).                                                                                                | × |
| Gas (Hybrid) | JetRadioEmissionShockingIntegrals       | The integrals over the shocking rates, used for radio emission modeling, in physical frame. The first integral corresponds to the electron integral, the second to the magnetic field integral, and the last to the 'minimum' auxilliary integral (see documentation). | × |
| Gas (Hybrid) | KickedByJetFeedback                     | Flags the particles that have been directly kicked by an AGN jet feedback event at some point in the past. If greater than 0, contains the number of individual events                                                                                                 | × |
| Gas (Hybrid) | LastAGNJetFeedbackInitialVolumes        | The physical volumes the particles had the last time they were heated by AGN.                                                                                                                                                                                          | × |
| Gas (Hybrid) | LastAGNJetFeedbackScaleFactors          | Scale-factors at which the particles were last hit by jet feedback. -1 if a particle has never been hit by feedback                                                                                                                                                    | ✓ |
| Gas (Hybrid) | LastAGNJetKickBHId                      | The id of the BH that last kicked this particle.                                                                                                                                                                                                                       | × |
| Gas (Hybrid) | LastAGNJetKickMode                      | The accretion/feedback mode the BH was in when it kicked this particle. 0 corresponds to the thick disc, 1 to the thin disc and 2 to the slim disc.                                                                                                                    | × |

|              |                                  |                                                                                                                                                                                                                                                       |   |
|--------------|----------------------------------|-------------------------------------------------------------------------------------------------------------------------------------------------------------------------------------------------------------------------------------------------------|---|
| Gas (Hybrid) | LastAGNJetKickVelocities         | Kick velocity at last AGN jet event.                                                                                                                                                                                                                  | × |
| Gas (Hybrid) | WeightedJetInjectionScaleFactors | The integral of the scale factor times shocking rate (injection rate of relativistic electrons), in physical frame. Once divided by a similar integral over the shocking rate, we get a weighted scale factor of when most of the injection occurred. | × |
| Stars        | Ages                             | Ages of the stars.                                                                                                                                                                                                                                    | ✓ |
| Stars        | AveragedStarFormationRates       | Star formation rates of the particles averaged over the period set by the first two snapshot triggers when the particle was still a gas particle.                                                                                                     | ✓ |
| Stars        | BirthDensities                   | Physical densities at the time of birth of the gas particles that turned into stars (note that we store the physical density at the birth redshift, no conversion is needed)                                                                          | ✓ |
| Stars        | BirthScaleFactors                | Scale-factors at which the stars were born                                                                                                                                                                                                            | ✓ |
| Stars        | BirthTemperatures                | Temperatures at the time of birth of the gas particles that turned into stars                                                                                                                                                                         | ✓ |
| Stars        | BirthVelocityDispersions         | Physical velocity dispersions (3D) squared at the birth time of the gas particles that turned into stars, this is the velocity dispersion of the total velocity (peculiar velocity + Hubble flow, $a H x + a (dx/dt)$ ).                              | ✓ |
| Stars        | Coordinates                      | Co-moving position of the particles                                                                                                                                                                                                                   | ✓ |
| Stars        | DensitiesAtLastAGNEvent          | Physical density (not subgrid) of the gas at the last AGN feedback event that hit the particles when they were still gas particles. -1 if the particles have never been heated.                                                                       | × |
| Stars        | DensitiesAtLastSupernovaEvent    | Physical density (not subgrid) of the gas at the last SN (type-II or type-Ia) thermal feedback event that hit the particles when they were still gas particles. -1 if the particles have never been heated.                                           | × |
| Stars        | ElementMassFractions             | Fractions of the particles' masses that are in the given element                                                                                                                                                                                      | ✓ |
| Stars        | EnergiesReceivedFromAGNFeedback  | Total amount of thermal energy from AGN feedback events received by the particles when the particles were still gas particles.                                                                                                                        | × |

|       |                                      |                                                                                                                                                                                            |   |
|-------|--------------------------------------|--------------------------------------------------------------------------------------------------------------------------------------------------------------------------------------------|---|
| Stars | FOFGroupIDs                          | Friends-Of-Friends ID of the group the particles belong to                                                                                                                                 | ✓ |
| Stars | InitialMasses                        | Masses of the star particles at birth time                                                                                                                                                 | ✓ |
| Stars | IronMassFractionsFromSNIa            | Fractions of the particles' masses that are in iron produced by SNIa stars                                                                                                                 | ✓ |
| Stars | LastAGNFeedbackScaleFactors          | Scale-factors at which the particles were last hit by AGN feedback when they were still gas particles. -1 if a particle has never been hit by feedback                                     | ✓ |
| Stars | LastEnergiesReceivedFromAGNFeedback  | The energy the particles received the last time they were heated by AGN feedback while they were still gas particles.                                                                      | × |
| Stars | LastFOFHaloMasses                    | Masses of the last FOF haloes the particles where part of when they were still a gas particle. -1 if the particle has never been in a FOF group                                            | ✓ |
| Stars | LastFOFHaloMassesScaleFactors        | Scale-factors at which the particle was last in a FOF group when they were still a gas particle                                                                                            | ✓ |
| Stars | LastKineticEarlyFeedbackScaleFactors | Scale-factors at which the particles were last hit by kinetic early feedback when they were still gas particles. -1 if a particle has never been hit by feedback                           | ✓ |
| Stars | LastSNIKineticFeedbackScaleFactors   | Scale-factors at which the particles were last hit by SNII kinetic feedback when they were still gas particles. -1 if a particle has never been hit by feedback                            | × |
| Stars | LastSNIKineticFeedbackvkick          | Physical kick velocity at last SNII kinetic feedback event when the stellar particles were kicked with when they were still gas particles. -1 if a particle has never been hit by feedback | × |
| Stars | LastSNIIThermalFeedbackScaleFactors  | Scale-factors at which the particles were last hit by SNII thermal feedback when they were still gas particles. -1 if a particle has never been hit by feedback                            | ✓ |
| Stars | LastSNIaThermalFeedbackScaleFactors  | Scale-factors at which the particles were last hit by SNIa thermal feedback when they were still gas particles. -1 if a particle has never been hit by feedback                            | ✓ |



|       |                                 |                                                                                                                                                                                                                                                                                                                                                                                                                                                                                                                                                                                   |   |
|-------|---------------------------------|-----------------------------------------------------------------------------------------------------------------------------------------------------------------------------------------------------------------------------------------------------------------------------------------------------------------------------------------------------------------------------------------------------------------------------------------------------------------------------------------------------------------------------------------------------------------------------------|---|
| Stars | Luminosities                    | Rest-frame dust-free AB-luminosities of the star particles in the GAMA bands. These were computed using the BC03 (GALAXEV) models convolved with different filter bands and interpolated in log-log ( $f(\log(Z), \log(\text{age})) = \log(\text{flux})$ ) as used in the dust-free modelling of Trayford et al. (2015). The luminosities are given in dimensionless units. They have been divided by 3631 Jy already, i.e. they can be turned into absolute AB-magnitudes (rest-frame absolute maggies) directly by applying $-2.5 \log_{10}(L)$ without additional corrections. | ✓ |
| Stars | MassFractionsFromAGB            | Fractions of the particles' masses that have been produced by AGB stars                                                                                                                                                                                                                                                                                                                                                                                                                                                                                                           | ✓ |
| Stars | MassFractionsFromCEJSN          | Fractions of the particles' masses that have been produced by common-envelop jets SN events                                                                                                                                                                                                                                                                                                                                                                                                                                                                                       | ✓ |
| Stars | MassFractionsFromCollapsar      | Fractions of the particles' masses that have been produced by collapsar events                                                                                                                                                                                                                                                                                                                                                                                                                                                                                                    | ✓ |
| Stars | MassFractionsFromNSM            | Fractions of the particles' masses that have been produced by neutron star merger events                                                                                                                                                                                                                                                                                                                                                                                                                                                                                          | ✓ |
| Stars | MassFractionsFromSNII           | Fractions of the particles' masses that have been produced by SNII stars                                                                                                                                                                                                                                                                                                                                                                                                                                                                                                          | ✓ |
| Stars | MassFractionsFromSNIa           | Fractions of the particles' masses that have been produced by SNIa stars                                                                                                                                                                                                                                                                                                                                                                                                                                                                                                          | ✓ |
| Stars | Masses                          | Masses of the particles at the current point in time (i.e. after stellar losses)                                                                                                                                                                                                                                                                                                                                                                                                                                                                                                  | ✓ |
| Stars | MaximalSNIIKineticFeedbackvkick | Maximal physical kick velocity in SNII kinetic feedback when the stellar particles were kicked with when they were still gas particles. -1 if a particle has never been hit by feedback                                                                                                                                                                                                                                                                                                                                                                                           | ✗ |
| Stars | MaximalTemperatureScaleFactors  | Scale-factors at which the maximal temperature was reached                                                                                                                                                                                                                                                                                                                                                                                                                                                                                                                        | ✓ |
| Stars | MaximalTemperatures             | Maximal temperatures ever reached by the particles before they got converted to stars                                                                                                                                                                                                                                                                                                                                                                                                                                                                                             | ✓ |
| Stars | MetalMassFractions              | Fractions of the particles' masses that are in metals                                                                                                                                                                                                                                                                                                                                                                                                                                                                                                                             | ✓ |
| Stars | MetalMassFractionsFromAGB       | Fractions of the particles' masses that are in metals produced by AGB stars                                                                                                                                                                                                                                                                                                                                                                                                                                                                                                       | ✓ |

|       |                                          |                                                                                                                                                                                                                                                                                                              |   |
|-------|------------------------------------------|--------------------------------------------------------------------------------------------------------------------------------------------------------------------------------------------------------------------------------------------------------------------------------------------------------------|---|
| Stars | MetalMassFractionsFromSNII               | Fractions of the particles' masses that are in metals produced by SNII stars                                                                                                                                                                                                                                 | ✓ |
| Stars | MetalMassFractionsFromSNIa               | Fractions of the particles' masses that are in metals produced by SNIa stars                                                                                                                                                                                                                                 | ✓ |
| Stars | ParticleIDs                              | Unique ID of the particles                                                                                                                                                                                                                                                                                   | ✓ |
| Stars | Potentials                               | Gravitational potentials of the particles                                                                                                                                                                                                                                                                    | ✓ |
| Stars | ProgenitorParticleIDs                    | Progenitor ID of the gas particle that became this star. If this particle is the result of one (or many) splitting events, this ID corresponds to the ID of the particle in the initial conditions that its lineage can be traced back to. If the particle was never split, this is the same as ParticleIDs. | ✓ |
| Stars | SNIIFeedbackEnergyFractions              | Fractions of the canonical feedback energy that was used for the stars' SNII feedback events                                                                                                                                                                                                                 | ✓ |
| Stars | SNIaRates                                | SNIa rate averaged over the last enrichment timestep                                                                                                                                                                                                                                                         | ✓ |
| Stars | SmoothingLengths                         | Co-moving smoothing lengths (FWHM of the kernel) of the particles                                                                                                                                                                                                                                            | ✓ |
| Stars | SplitCounts                              | Number of times the gas particle that turned into this star particle was split. Note that both particles that take part in the splitting have their counter incremented.                                                                                                                                     | ✓ |
| Stars | SplitTrees                               | Binary tree describing splitting events. Particles that keep the original ID have a value of zero in a splitting event, whereas particles given a new ID have a value of one.                                                                                                                                | ✓ |
| Stars | TemperatureIncreasesAtLastAGNEvent       | The increase in temperature of the gas at the last AGN feedback event that hit the particles when they were still gas particles. -1 if the particles have never been heated.                                                                                                                                 | ✓ |
| Stars | TemperatureIncreasesAtLastSupernovaEvent | The increase in temperature of the gas at the last SN (type-II or type-Ia) thermal feedback event that hit the particles when they were still gas particles. -1 if the particles have never been heated.                                                                                                     | ✓ |
| Stars | Velocities                               | Peculiar velocities of the particles. This is a $\ast dx/dt$ where x is the co-moving position of the particles.                                                                                                                                                                                             | ✓ |

---

|                |                                 |                                                                                                                                                                        |   |
|----------------|---------------------------------|------------------------------------------------------------------------------------------------------------------------------------------------------------------------|---|
| Stars (Hybrid) | EnergiesReceivedFromJetFeedback | Total amount of kinetic energy from AGN jet feedback events received by the particles while they were still gas particles.                                             | ✓ |
| Stars (Hybrid) | KickedByJetFeedback             | Flags the particles that have been directly kicked by an AGN jet feedback event at some point in the past. If greater than 0, contains the number of individual events | ✓ |
| Stars (Hybrid) | LastAGNJetFeedbackScaleFactors  | Scale-factors at which the particles were last hit by jet feedback while they were still gas particles. -1 if a particle has never been hit by feedback                | ✓ |
| Stars (Hybrid) | LastAGNJetKickBHId              | The id of the BH that last kicked this particle.                                                                                                                       | ✓ |
| Stars (Hybrid) | LastAGNJetKickMode              | The accretion/feedback mode the BH was in when it kicked this particle. 0 corresponds to the thick disc, 1 to the thin disc and 2 to the slim disc.                    | ✓ |
| Stars (Hybrid) | LastAGNJetKickVelocities        | Kick velocity at last AGN jet event.                                                                                                                                   | ✓ |
| Stars (GCs)    | BirthCircularFrequency          | Circular frequency at time of star formation                                                                                                                           | × |
| Stars (GCs)    | BirthEpicyclicFrequency         | Epicyclic frequency at time of star formation                                                                                                                          | × |
| Stars (GCs)    | BirthGasFraction                | Local gas fraction (within cell) at time of star formation                                                                                                             | × |
| Stars (GCs)    | BirthToomreMass                 | Local Toomre mass at formation                                                                                                                                         | × |
| Stars (GCs)    | ClusterFormationEfficiency      | Fraction of star formation which occurs in bound star clusters                                                                                                         | × |
| Stars (GCs)    | ClusterMassTotal                | Sum of surviving star cluster masses                                                                                                                                   | ✓ |
| Stars (GCs)    | ClusterTruncationMass           | Exponential truncation of star cluster initial mass function (Mcstar)                                                                                                  | × |
| Stars (GCs)    | DisruptionScaleFactors          | Scale-factors at which clusters became disrupted (-1 if surviving)                                                                                                     | × |
| Stars (GCs)    | FgasCellWidth                   | Cell width at point of gas fraction calculation                                                                                                                        | × |
| Stars (GCs)    | InitialClusterMassEvoLim        | Sum of initial star cluster masses above evolution mass limit                                                                                                          | × |
| Stars (GCs)    | InitialClusterMassTotal         | Sum of initial star cluster masses                                                                                                                                     | × |
| Stars (GCs)    | InitialMasses                   | Initial masses of clusters tagged to particle                                                                                                                          | × |
| Stars (GCs)    | InitialNumberOfClusters         | Number of star clusters tried to form in total                                                                                                                         | ✓ |
| Stars (GCs)    | InitialNumberOfClustersEvoLim   | Number of star clusters formed above evolution mass limit                                                                                                              | × |

|             |                           |                                                                                                                                                                                       |   |
|-------------|---------------------------|---------------------------------------------------------------------------------------------------------------------------------------------------------------------------------------|---|
| Stars (GCs) | MassLossShocks            | Cluster mass lost to tidal shocks                                                                                                                                                     | × |
| Stars (GCs) | Masses                    | Masses of clusters tagged to particle                                                                                                                                                 | × |
| Stars (GCs) | NumberOfClusters          | Surviving number of subgrid star clusters                                                                                                                                             | × |
| Stars (GCs) | SubgridFieldMass          | Subgrid field mass component of star particle                                                                                                                                         | ✓ |
| Stars (GCs) | ToomreCollapseFraction    | Fraction of Toomre mass which can collapse to a GMC                                                                                                                                   | × |
| Stars (GCs) | TidalTensors              | Components of co-moving the tidal tensor (Hessian matrix of the gravitational potential). Since the matrix is symmetric, only 6 values per tensor are stored (xx, yy, zz, xy, xz, yz) | ✓ |
| Black holes | AGNTotalInjectedEnergies  | Total (cumulative) physical energies injected into gas particles in AGN feedback.                                                                                                     | ✓ |
| Black holes | AccretedAngularMomenta    | Physical angular momenta that the black holes have accumulated through subgrid accretion.                                                                                             | ✓ |
| Black holes | AccretionBoostFactors     | Multiplicative factors by which the Bondi-Hoyle-Lyttleton accretion rates have been increased by the density-dependent Booth & Schaye (2009) accretion model.                         | ✓ |
| Black holes | AccretionLimitedTimeSteps | Accretion-limited time steps of black holes. The actual time step of the particles may differ due to the minimum allowed value.                                                       | ✓ |
| Black holes | AccretionRates            | Physical instantaneous accretion rates of the particles                                                                                                                               | ✓ |
| Black holes | AveragedAccretionRates    | Accretion rates of the black holes averaged over the period set by the first two snapshot triggers                                                                                    | ✓ |
| Black holes | Coordinates               | Co-moving position of the particles                                                                                                                                                   | ✓ |
| Black holes | CumulativeNumberOfSeeds   | Total number of BH seeds that have merged into this black hole                                                                                                                        | ✓ |
| Black holes | DustMasses                | Mass contents of the BH particles in a given dust grain species                                                                                                                       | ✓ |
| Black holes | DynamicalMasses           | Dynamical masses of the particles                                                                                                                                                     | ✓ |
| Black holes | EddingtonFractions        | Accretion rates of black holes in units of their Eddington rates. This is based on the unlimited accretion rates, so these fractions can be above the limiting $f_{\text{Edd}}$ .     | ✓ |

|             |                           |                                                                                                                                                                                                                                                                          |   |
|-------------|---------------------------|--------------------------------------------------------------------------------------------------------------------------------------------------------------------------------------------------------------------------------------------------------------------------|---|
| Black holes | ElementMasses             | Mass contents of the BH particles in a given element                                                                                                                                                                                                                     | ✓ |
| Black holes | ElementMassesDiffuse      | Masses of the BH that are in the given element and were in the gas phase when accreted                                                                                                                                                                                   | ✓ |
| Black holes | EnergyReservoirs          | Physcial energy contained in the feedback reservoir of the particles                                                                                                                                                                                                     | ✓ |
| Black holes | FOFGroupIDs               | Friends-Of-Friends ID of the group the particles belong to                                                                                                                                                                                                               | ✓ |
| Black holes | FormationScaleFactors     | Scale-factors at which the BHs were formed                                                                                                                                                                                                                               | ✓ |
| Black holes | GWMassLosses              | Cumulative masses lost to GW via BH-BH mergers over the history of the black holes. This includes the mass loss from all the progenitors.                                                                                                                                | ✓ |
| Black holes | GasCircularVelocities     | Circular velocities of the gas around the black hole at the smoothing radius. This is $j / h_{\text{BH}}$ , where $j$ is the smoothed, peculiar specific angular momentum of gas around the black holes, and $h_{\text{BH}}$ is the smoothing length of each black hole. | ✓ |
| Black holes | GasCurlVelocities         | Velocity curl (3D) of the gas particles around the black holes.                                                                                                                                                                                                          | ✓ |
| Black holes | GasDensities              | Co-moving densities of the gas around the particles                                                                                                                                                                                                                      | ✓ |
| Black holes | GasRelativeVelocities     | Peculiar relative velocities of the gas particles around the black holes. This is $a * dx/dt$ where $x$ is the co-moving position of the particles.                                                                                                                      | ✓ |
| Black holes | GasSoundSpeeds            | Co-moving sound-speeds of the gas around the particles                                                                                                                                                                                                                   | ✓ |
| Black holes | GasTemperatures           | Temperature of the gas surrounding the black holes.                                                                                                                                                                                                                      | ✓ |
| Black holes | GasVelocityDispersions    | Velocity dispersion (3D) of the gas particles around the black holes. This is $a\sqrt{\langle  dx/dt ^2 \rangle - \langle  dx/dt  \rangle^2}$ where $x$ is the co-moving position of the particles relative to the black holes.                                          | ✓ |
| Black holes | IronMassesFromSNIa        | Masses of the BH particles in iron that have been produced by SNIa stars                                                                                                                                                                                                 | ✓ |
| Black holes | IronMassesFromSNIaDiffuse | Masses of the BH particles in iron that have been produced by SNIa stars and were in the gas phase when accreted                                                                                                                                                         | ✓ |

|             |                                       |                                                                                                                                                                                                        |   |
|-------------|---------------------------------------|--------------------------------------------------------------------------------------------------------------------------------------------------------------------------------------------------------|---|
| Black holes | LastAGNFeedbackScaleFactors           | Scale-factors at which the black holes last had an AGN event.                                                                                                                                          | ✓ |
| Black holes | LastHighEddingtonFractionScaleFactors | Scale-factors at which the black holes last reached a large Eddington ratio. -1 if never reached.                                                                                                      | ✓ |
| Black holes | LastMajorMergerScaleFactors           | Scale-factors at which the black holes last had a major merger.                                                                                                                                        | ✓ |
| Black holes | LastMinorMergerScaleFactors           | Scale-factors at which the black holes last had a minor merger.                                                                                                                                        | ✓ |
| Black holes | LastRepositionVelocities              | Physical speeds at which the black holes repositioned most recently. This is 0 for black holes that have never repositioned, or if the simulation has been run without prescribed repositioning speed. | ✓ |
| Black holes | MassesFromAGB                         | Masses of the BH particles that have been produced by AGB stars                                                                                                                                        | ✓ |
| Black holes | MassesFromCEJSN                       | Masses of the BH particles in europium that have been produced by common-envelope jets SN events                                                                                                       | ✓ |
| Black holes | MassesFromCollapsar                   | Masses of the BH particles in europium that have been produced by collapsar events                                                                                                                     | ✓ |
| Black holes | MassesFromNSM                         | Masses of the BH particles in europium that have been produced by neutron star merger events                                                                                                           | ✓ |
| Black holes | MassesFromSNII                        | Masses of the BH particles that have been produced by SNII stars                                                                                                                                       | ✓ |
| Black holes | MassesFromSNIa                        | Masses of the BH particles that have been produced by SNIa stars                                                                                                                                       | ✓ |
| Black holes | MetalMasses                           | Mass contents of the BH particles in a metals                                                                                                                                                          | ✓ |
| Black holes | MetalMassesFromAGB                    | Masses of the BH particles in metals that have been produced by AGB stars                                                                                                                              | ✓ |
| Black holes | MetalMassesFromSNII                   | Masses of the BH particles in metals that have been produced by SNII stars                                                                                                                             | ✓ |
| Black holes | MetalMassesFromSNIa                   | Masses of the BH particles in metals that have been produced by SNIa stars                                                                                                                             | ✓ |
| Black holes | MinimalTimeBinScaleFactors            | Scale-factors at which the minimal time-bin was reached                                                                                                                                                | ✓ |
| Black holes | MinimalTimeBins                       | Minimal Time Bins reached by the black holes                                                                                                                                                           | ✓ |

|             |                       |                                                                                                                                                                                                                                                                                                                |   |
|-------------|-----------------------|----------------------------------------------------------------------------------------------------------------------------------------------------------------------------------------------------------------------------------------------------------------------------------------------------------------|---|
| Black holes | NumberOfAGNEvents     | Integer number of AGN events the black hole has had so far (the number of time steps in which the BH did AGN feedback).                                                                                                                                                                                        | ✓ |
| Black holes | NumberOfGasNeighbours | Integer number of gas neighbour particles within the black hole kernels.                                                                                                                                                                                                                                       | ✓ |
| Black holes | NumberOfHeatingEvents | Integer number of (thermal) energy injections the black hole has had so far. This counts each heated gas particle separately, and so can increase by more than one during a single time step.                                                                                                                  | ✓ |
| Black holes | NumberOfMergers       | Number of mergers the black holes went through. This does not include the number of mergers accumulated by any merged black hole.                                                                                                                                                                              | ✓ |
| Black holes | NumberOfRepositions   | Number of repositioning events the black holes went through. This does not include the number of reposition events accumulated by any merged black holes.                                                                                                                                                      | ✓ |
| Black holes | NumberOfTimeSteps     | Total number of time steps at which the black holes were active.                                                                                                                                                                                                                                               | ✓ |
| Black holes | ParticleIDs           | Unique ID of the particles                                                                                                                                                                                                                                                                                     | ✓ |
| Black holes | Potentials            | Gravitational potentials of the particles                                                                                                                                                                                                                                                                      | ✓ |
| Black holes | ProgenitorParticleIDs | Progenitor ID of the gas particle that became the seed BH. If this particle is the result of one (or many) splitting events, this ID corresponds to the ID of the particle in the initial conditions that its lineage can be traced back to. If the particle was never split, this is the same as ParticleIDs. | ✓ |
| Black holes | SmoothingLengths      | Co-moving smoothing lengths (FWHM of the kernel) of the particles                                                                                                                                                                                                                                              | ✓ |
| Black holes | SplitCounts           | Number of times the gas particle that became this BH seed was split. Note that both particles that take part in the splitting have their counter incremented.                                                                                                                                                  | ✓ |
| Black holes | SplitTrees            | Binary tree describing splitting events prior to BH seeding. Particles that keep the original ID have a value of zero in a splitting event, whereas particles given a new ID have a value of one.                                                                                                              | ✓ |
| Black holes | SubgridMasses         | Subgrid masses of the particles                                                                                                                                                                                                                                                                                | ✓ |

|                      |                                |                                                                                                                                                                                                                                                                    |   |
|----------------------|--------------------------------|--------------------------------------------------------------------------------------------------------------------------------------------------------------------------------------------------------------------------------------------------------------------|---|
| Black holes          | SwallowedAngularMomenta        | Physical angular momenta that the black holes have accumulated by swallowing gas particles.                                                                                                                                                                        | ✓ |
| Black holes          | TotalAccretedMasses            | Total mass accreted onto the main progenitor of the black holes since birth. This does not include any mass accreted onto any merged black holes.                                                                                                                  | ✓ |
| Black holes          | Velocities                     | Peculiar velocities of the particles. This is a $\dot{x}$ where $x$ is the co-moving position of the particles.                                                                                                                                                    | ✓ |
| Black holes (Hybrid) | AGNTotalInjectedEnergiesByMode | The total energy injected in the thermal AGN feedback mode, including the contributions of both radiation and wind feedback, split by accretion mode. The components correspond to the thermal energy dumped in the thick, thin and slim disc modes, respectively. | ✓ |
| Black holes (Hybrid) | AccretionModes                 | Accretion flow regime. 0 - Thick disk, 1 - Thin disk, 2 - Slim disk                                                                                                                                                                                                | ✓ |
| Black holes (Hybrid) | AngularMomentumDirections      | Direction of the black hole spin vector, normalised to unity.                                                                                                                                                                                                      | ✓ |
| Black holes (Hybrid) | CosAccretionDiskAngle          | Cosine of the angle between the spin vector and the accreting gas angular momentum.                                                                                                                                                                                | ✓ |
| Black holes (Hybrid) | InjectedJetEnergies            | Total jet energy injected into AGN surroundings.                                                                                                                                                                                                                   | ✓ |
| Black holes (Hybrid) | InjectedJetEnergiesByMode      | The total energy injected in the kinetic jet AGN feedback mode, split by accretion mode. The components correspond to the jet energy dumped in the thick, thin and slim disc modes, respectively.                                                                  | ✓ |
| Black holes (Hybrid) | JetEfficiencies                | Jet power divided by accretion rate.                                                                                                                                                                                                                               | ✓ |
| Black holes (Hybrid) | JetReservoir                   | Total jet energy waiting to be released (once it grows large enough to kick a single particle).                                                                                                                                                                    | ✓ |
| Black holes (Hybrid) | JetTimeSteps                   | Jet-launching-limited time-steps of black holes.                                                                                                                                                                                                                   | ✓ |
| Black holes (Hybrid) | JetVelocities                  | The current jet velocities.                                                                                                                                                                                                                                        | ✓ |
| Black holes (Hybrid) | LastAGNJetScaleFactors         | Scale-factors at which the black holes last had an AGN jet event.                                                                                                                                                                                                  | ✓ |
| Black holes (Hybrid) | NumberOfAGNJetEvents           | Integer number of AGN jet launching events the black hole has had (the number of times the BH did AGN jet feedback)                                                                                                                                                | ✓ |
| Black holes (Hybrid) | NumberOfJetParticlesLaunched   | Integer number of (kinetic) energy injections the black hole has had so far                                                                                                                                                                                        | ✓ |



|                      |                           |                                                                                                                                                                                                                 |   |
|----------------------|---------------------------|-----------------------------------------------------------------------------------------------------------------------------------------------------------------------------------------------------------------|---|
| Black holes (Hybrid) | RadiatedEnergiesByMode    | The total energy launched into radiation by the black holes, split by accretion mode. The components correspond to the radiative energy dumped in the thick, thin and slim disc modes, respectively.            | ✓ |
| Black holes (Hybrid) | RadiativeEfficiencies     | AGN luminosity divided by accretion rate.                                                                                                                                                                       | ✓ |
| Black holes (Hybrid) | Spins                     | Dimensionless spins of the black holes. Negative values indicate retrograde accretion.                                                                                                                          | ✓ |
| Black holes (Hybrid) | TotalAccretedMassesByMode | The total accreted mass in each accretion mode. The components to the mass accreted in the thick, thin and slim disc modes, respectively.                                                                       | ✓ |
| Black holes (Hybrid) | TotalRadiatedEnergies     | The total energy launched into radiation by the black holes, in all accretion modes.                                                                                                                            | ✓ |
| Black holes (Hybrid) | TotalWindEnergies         | The total energy launched into accretion disc winds by the black holes, in all accretion modes.                                                                                                                 | ✓ |
| Black holes (Hybrid) | WindEfficiencies          | The wind efficiencies of the black holes.                                                                                                                                                                       | ✓ |
| Black holes (Hybrid) | WindEnergiesByMode        | The total energy launched into accretion disc winds by the black holes, split by accretion mode. The components correspond to the radiative energy dumped in the thick, thin and slim disc modes, respectively. | ✓ |

---
